# Supplementary material for: Bag All You Need: Learning a Generalizable Bagging Strategy for Heterogeneous Objects
Source: arXiv:2210.09997 source file (2023-10-01)
Supplement: Supplementary file 1 [file appendix.tex]

\section*{{\color{orange}APPENDIX}}
\label{sec:appendix}
\begin{figure}[H]
    \centering
    \includegraphics[width= 0.97\linewidth]{figure/Appendix_1.pdf}
    \caption{\textbf{Heuristic rearrangement and lifting strategies in the real world:} The pick point is chosen from the blue region and the place point is denoted by the red circle. The green circles denote the lift points}  
    \label{fig:objects}
    % https://docs.google.com/drawings/d/1zNEGCZqv7XL7kgOR1-nZhS_rYTJ2j-JcN5DQLRszKGM/edit
\end{figure}

% \begin{figure}[H]
%     \centering
%     \includegraphics[width= 0.97\linewidth]{figure/Appendix_2.pdf}
%     \caption{Explanation of some terminologies}  
%     \label{fig:objects}
%     % https://docs.google.com/drawings/d/1E1g8EudqivTmoL_97c266yelHAxCh1s_n5C0tsWYgyM/edit
% \end{figure}
